# Supplementary material for: Navigating Semantic Drift in Task-Agnostic Class-Incremental Learning
Source: arXiv:2502.07560 source file (2025-02-17)
Supplement: Supplementary file 1 [file appendix.tex]

% \appendix
% \onecolumn
% \section{You \emph{can} have an appendix here.}

% You can have as much text here as you want. The main body must be at most $8$ pages long.
% For the final version, one more page can be added.
% If you want, you can use an appendix like this one.  

% The $\mathtt{\backslash onecolumn}$ command above can be kept in place if you prefer a one-column appendix, or can be removed if you prefer a two-column appendix.  Apart from this possible change, the style (font size, spacing, margins, page numbering, etc.) should be kept the same as the main body.

% \input{sections/fig_lambda}
% \input{sections/fig_r}
% \input{sections/fig_s}
